# Supplementary material for: Weakly supervised multimodal segmentation of acoustic borehole images with depth-aware cross-attention
Source: arXiv:2603.20729 source file (2026-03-21)
Supplement: Supplementary file 1 [file suplementarmaterial.tex]

\documentclass[11pt]{article}
\usepackage[utf8]{inputenc}
\usepackage[T1]{fontenc}
\usepackage{geometry}
\geometry{a4paper, margin=1in}
\usepackage{graphicx}
\usepackage{amsmath, amssymb}
\usepackage{caption}
\usepackage{booktabs}
\usepackage{multirow}
\usepackage{hyperref}

% --- Nature SI Requirement: Separate Numbering ---

\title{\textbf{Supplementary Information for:}\\ Weakly supervised multimodal segmentation of acoustic borehole images with depth-aware cross-attention}
\author{Jose Luis Lima de Jesus Silva}
\date{}

\begin{document}

\maketitle

\section{Supplementary Tables}
\label{sec:supp_tables}

\begin{table}[htbp]
\centering
\caption{\textbf{Descriptive statistics of the selected aligned log channels used by the multimodal model in the initial Antilope25 interval.} Each channel was independently normalized before visualization and model input. The values represent relative within-channel variation rather than directly comparable absolute physical units.}
\label{tab:S1_selected_log_statistics_antilope25}
\begin{tabular}{lcc}
\toprule
Channel & Mean & Standard deviation \\
\midrule
Caliper (CAL) & 0.4119 & 0.3573 \\
Gamma Ray (GR) & 0.2692 & 0.2170 \\
Bulk Density (DEN) & 0.4707 & 0.3313 \\
Neutron Porosity (NEU) & 0.4810 & 0.3312 \\
Compressional Slowness (DTC) & 0.3921 & 0.2845 \\
Deep Resistivity (RES90) & 0.5013 & 0.2981 \\
\bottomrule
\end{tabular}
\end{table}

\begin{table}[htbp]
\centering
\caption{\textbf{Quantitative summary of the initial Antilope25 interval results.} Agreement values are reported with respect to the pseudo-label reference and the denoised thresholding result. As the reference is weakly supervised rather than manually annotated ground truth, these values represent internal consistency measures.}
\label{tab:S2_initial_antilope25_metrics}
\begin{tabular}{lcc}
\toprule
Method & Agreement vs pseudo-labels & Agreement vs denoised thresholding \\
\midrule
Raw thresholding & 0.6002 & 0.7621 \\
Denoised thresholding & 0.7456 & 1.0000 \\
AE + KMeans clustering & 0.4212 & 0.4819 \\
Refined segmentation, image only & 0.8938 & 0.7015 \\
Refined segmentation, multimodal & \textbf{0.9262} & 0.7337 \\
\bottomrule
\end{tabular}
\end{table}

\begin{table}[htbp]
\centering
\caption{\textbf{Mean agreement values from the compact cross-well screening stage.} Agreement is reported with respect to the pseudo-label reference. The image-only refiner and the simple concatenation-based multimodal refiner perform similarly on average, prompting the development of the depth-aware cross-attention mechanism.}
\label{tab:S3_compact_screening_summary}
\begin{tabular}{lc}
\toprule
Method & Mean agreement vs pseudo-labels \\
\midrule
Raw thresholding & 0.6670 \\
Denoised thresholding & 0.7223 \\
AE + KMeans clustering & 0.5201 \\
Refined segmentation, image only & \textbf{0.8349} \\
Refined segmentation, multimodal (Concat) & 0.8305 \\
\bottomrule
\end{tabular}
\end{table}

\begin{table}[htbp]
\centering
\caption{\textbf{Method-level agreement values for the representative heavy-rerun case studies.} Agreement is reported with respect to the pseudo-label reference. These intervals were selected from different wells and depth regimes to represent distinct morphological challenges. The ID ranges in the first column refer to the row indices of the extracted slices.}
\label{tab:S4_heavy_case_studies}
\begin{tabular}{p{4.5cm}ccccc}
\toprule
Interval & Raw & AE $\rightarrow$ & AE + & Image & Multimodal \\
(Well, Regime, Row Indices) & Otsu & Otsu & KMeans & only & (Concat) \\
\midrule
Botorosa47 \newline (Mid, 40231--40831) & 0.7309 & 0.7595 & 0.5833 & 0.8664 & \textbf{0.9133} \\
\addlinespace
Antilope25 \newline (Deep, 219035--219635) & 0.8638 & 0.9285 & 0.6140 & \textbf{0.9524} & 0.9445 \\
\addlinespace
Antilope25 \newline (Mid, 109517--110117) & 0.6494 & 0.6577 & 0.5782 & \textbf{0.8105} & 0.5809 \\
\bottomrule
\end{tabular}
\end{table}

\begin{table}[htbp]
\centering
\caption{\textbf{Compact benchmark summary for the depth-aware multimodal refiners.} Agreement is reported with respect to the pseudo-label reference across 58 evaluation intervals. The progression demonstrates that selective, depth-aware fusion fundamentally outperforms simple channel concatenation.}
\label{tab:S5_phase4_benchmark}
\begin{tabular}{lc}
\toprule
Method & Mean agreement vs pseudo-labels \\
\midrule
Raw Otsu & 0.6234 \\
AE $\rightarrow$ Otsu & 0.7078 \\
AE + KMeans & 0.4745 \\
M-TGS image-only & 0.7387 \\
Multimodal (Concat) & 0.7550 \\
DCA & 0.8098 \\
G-DCA & 0.8201 \\
CG-DCA & \textbf{0.8603} \\
\bottomrule
\end{tabular}
\end{table}

\begin{table}[htbp]
\centering
\caption{\textbf{Case-level structural comparison metrics for the selected Phase~4 intervals.} Agreement is reported against the pseudo-label reference after class alignment. Off-diagonal mass is computed from the corresponding confusion matrix, so lower values indicate stronger class-wise consistency. For DCA, G-DCA, and CG-DCA, the final two columns report stepwise changes relative to the preceding multimodal method in the sequence.}
\label{tab:S6_phase4_selected_case_metrics}
\small
\begin{tabular}{llcccc}
\toprule
Case & Method & Agreement & Off-diag. & Changed & Low-conf. \\
\midrule
\multirow{4}{*}{Coala88}
& Concat multimodal & 0.9014 & 0.0986 &  &  \\
& DCA               & 0.9323 & 0.0677 & 0.0713 & 0.5850 \\
& G-DCA             & 0.9411 & 0.0589 & 0.0568 & 0.6121 \\
& CG-DCA            & 0.9739 & 0.0261 & 0.0569 & 0.5886 \\
\midrule
\multirow{4}{*}{Botorosa47}
& Concat multimodal & 0.8806 & 0.1194 &  &  \\
& DCA               & 0.9336 & 0.0664 & 0.0908 & 0.4928 \\
& G-DCA             & 0.9346 & 0.0654 & 0.0428 & 0.5702 \\
& CG-DCA            & 0.9568 & 0.0432 & 0.0614 & 0.5898 \\
\midrule
\multirow{4}{*}{Antilope25 top}
& Concat multimodal & 0.8991 & 0.1009 &  &  \\
& DCA               & 0.9702 & 0.0298 & 0.0878 & 0.5948 \\
& G-DCA             & 0.9765 & 0.0235 & 0.0191 & 0.7043 \\
& CG-DCA            & 0.9738 & 0.0262 & 0.0194 & 0.6706 \\
\bottomrule
\end{tabular}
\end{table}

\end{document}
